# Supplementary material for: Neural Network Approximations of PDEs Beyond Linearity: A Representational Perspective
Source: arXiv:2210.12101 source file (2023-03-27)
Supplement: Supplementary file 2 [file barron_recursion_lemma_proof.tex]

\subsection{Proof for Lemma~\ref{lemma:barron_norm_recursion}: 
Barron Norm Recursion}
\label{subsec:proof_of_barron_norm_recursion}
\begin{proof}
    Note that the update equation looks like, 
    \begin{align*}
        u_{t+1} 
            &= u_t - \eta (I - \Delta)^{-1} \op(u_t) \\
            &= u_t - \eta (I - \Delta)^{-1} \left(-\nabla \cdot \nabla L(\nabla u_t)\right)\\
            &= u_t - \eta (I - \Delta)^{-1} \left(-\sum_{i=1}^d \partial_i^2 L(\nabla u_t)\right) 
            \numberthis \label{eq:update_written_in_full}
    \end{align*}
    We first bound $\|u_t\|_{\fm}$. 
    
    Using results from Lemma~\ref{lemma:barron_norm_algebra}
    we have
    \begin{equation}
        \|\nabla u_t\|_{\barron}  = \max_{i \in [d]} 
            \|\partial_i u_t\|_{\barron} \leq  W_t\|u_t\|_{\barron}
    \end{equation}
    Similarly we can bound $\|\partial_i^2 L(\nabla u_t)\|_{\fm}$.  
    Note that since $u_t \in \Gamma_{W_t}$ 
    we have $\nabla u_t \in \Gamma_{W_t}$ and $L(\nabla u_t) \in \Gamma_{kW_t}$ 
    (from Assumption~\ref{assumption:2}).
    \begin{align*}
        \left\|(I - \Delta)^{-1} \left(-\sum_{i=1}^d \partial_i^2 L(\nabla u_t)\right)\right\|_{\fm} 
        &\stackrel{(i)}{\leq} \left\|-\sum_{i=1}^d \partial_i^2 L(\nabla u_t)\right\|_{\fm}\\
        &\stackrel{(ii)}{\leq}d^2\left\|\partial_i^2 L(\nabla u_t)\right\|_{\fm}\\
            &\leq d^2 (kW_t)^2 \|L(\nabla u_t)\|_{\fm} \\
            &\leq d^2 (kW_t)^2 A_{\tL} \|u_t\|^r_{\fm} 
    \end{align*}
    where we use the fact that for a function $h$, we have $\|(I - \Delta)^{-1}h\|_{\fm} \leq \|h\|_{\fm}$
    from Lemma~\ref{lemma:barron_norm_algebra} in $(i)$
    and the fact that $L(\nabla u_t) \in \Gamma_{kW_t}$ in $(ii)$.
    Using the result of \emph{Addition} 
    from Lemma~\ref{lemma:barron_norm_algebra}
    we have
    \begin{align*}
        \|u_t\|_{\fm} &\leq \|u_t\|_{\fm} + \left(\eta d^2 (kW_t)^2 A_{\tL}\right)\|u_t\|_{\fm}^r \\
            &\leq \left(1 + \eta d^2 (kW_t)^2 A_{\tL}\right)\|u_t\|_{\fm}^r 
    \end{align*}

    Now, to bound $\|u_{t+1}\|_{\barron}$, note that from 
    Assumption~\ref{assumption:2}
    we know that 
    $\|L \circ g\| \leq B_{\tL} \|g\|_{\fm}^q \|g\|_{\barron}^p$. 
    
    We start with bounding the following,
    \begin{align*}
        \left\|(I - \Delta)^{-1} \left(-\sum_{i=1}^d \partial_i^2 L(\nabla u_t)\right)\right\|_{\barron}
        &\leq 
        \left\|-\sum_{i=1}^d \partial_i^2 L(\nabla u_t)\right\|_{\barron} \\
        &\leq 
        d^2 \left\| L(\nabla u_t)\right\|_{\barron} \\
        &\leq 
        d^2 (kW_t)^2\left\| L(\nabla u_t)\right\|_{\barron} \\
        &\leq 
        d^2 (kW_t)^2B_{\tL} \|u_t\|_{\fm}^q \|u_t\|_{\barron}^{p}
    \end{align*}
    
    Using the result of \emph{Addition} 
    from Lemma~\ref{lemma:barron_norm_algebra}
    we have
    \begin{align*}
        \|u_t\|_{\barron} &\leq \|u_t\|_{\barron} + \eta d^2 (kW_t)^2B_{\tL} \|u_t\|_{\fm}^q \|u_t\|_{\barron}^{p}\\
            &\leq \left(1 + \eta d^2 (kW_t)^2 B_{\tL}\|u_t\|_{\fm}^q\right)\|u_t\|_{\barron}^p \\
    \end{align*}
\end{proof}
