# Supplementary material for: Neural Network Approximations of PDEs Beyond Linearity: A Representational Perspective
Source: arXiv:2210.12101 source file (2023-03-27)
Supplement: Supplementary file 3 [file proof_of_conversion_v1.tex]

\section{Proofs from Section~\ref{subsec:convergence_rate_of_sequence}}
\label{sec:appendix:proofs_for_convergence}

\subsection{Proof for Lemma~\ref{lemma:properties_of_EandL}}
\label{sec:appendix:proofs_for_results_for_variational_PDE}
\begin{proof}
    To show the first part, since
    $L:\R^d \to \R$
    is strongly convex and smooth, we have 
    
    $$\forall x \in \R^d, \lambda I_d \leq D^2L(x) \leq \Lambda I_d.$$
    % Since, from Assumption~\ref{assumption:1}
    % we know that 
    % $L(0) = 0$ and $\nabla L(0) = 0$, therefore 
    % we can bound $\nabla L(x)$  and $L(x)$ as,
    Therefore for any $x, y \in \R^d$
    we can bound 
    $\|\nabla L(x) - \nabla L(y)\|_2$
    \begin{align}
        \lambda \|x - y\|_2 &\leq \|\nabla L(x) - \nabla L(y)\|_2 
            \leq  \Lambda \|x - y\|_2.
    \end{align}
   Furthermore, taking $y = 0$  and from Assumption~\ref{assumption:2} we know $\nabla L(0) = 0$ 
   we get for all $x \in \R$
   \begin{align} 
        \lambda \|x\|^2_2 &\leq L(x)  \leq \Lambda \|x\|_2^2.
    \end{align}
    Therefore, we for any functions $u, v$ can bound $\op(u) - \op(v)$
    as follows,
    \begin{align*}
        \calE(u) - \calE(v) &=\int_\Omega L(\nabla u(x)) - L(\nabla v(x))dx \\
        &\leq \int_\Omega \Lambda \|\nabla u(x) - \nabla v(x)\|_2^2 dx\\
        &\leq \Lambda \|\nabla u - \nabla v \|_{\ll}^2
    \end{align*}
    Where we use the result for the $\ll$
    norm of a vector 
    valued function from Definition~\ref{def:lpnorm}.
    The proof for the lower norm follows similarly.

    In order to prove the point \emph{1.}
    we
    will use the following integration by parts identity,
    for functions $r:\Omega \to \R$ such that 
    and $s: \Omega \to \R$, and $r,s \in \h$,
    \begin{equation}
        \label{eq:change_of_variable_formula}
         \int_\Omega \frac{\partial r}{\partial x_i} s dx 
         = - \int_\Omega r \frac{\partial s}{\partial x_i} dx 
            + \int_{\partial \Omega}rs n d\Gamma
    \end{equation}
    where $n_i$ 
    is a normal at the boundary and 
    $d \Gamma$ is an infinitesimal element
    of the boundary $\partial \Omega$.
        
    Using the formula 
    in \eqref{eq:change_of_variable_formula} 
    for functions $u,v \in \h$
    where $u:\Omega \to \R$ 
    and $v: \Omega \to \R$, we have,
    \begin{align*}
        \langle \op(u), v\rangle_{\ll} &= \left\langle 
        -\nabla \cdot 
        \nabla L(\nabla u), v\right\rangle_{\ll}\\
        &= -\int_{\Omega} \nabla \cdot \nabla L(\nabla u) v dx \\
        &= -\int_{\Omega} \sum_{i=1}^d \frac{\partial \left(\nabla L(\nabla u)\right)_i}{\partial x_i} v dx\\
        &= \int_{\Omega} \sum_{i=1}^d  \left(\nabla L(\nabla u)\right)_i \frac{\partial v}{\partial x_i}  dx 
        + \int_\Omega \sum_{i=1}^d \left(\nabla L(\nabla u)\right)_i v n_i dx\\
        &= \int \nabla L(\nabla u) \cdot \nabla v dx
    \end{align*}
    where to get the final result,
    we use the fact that the function 
    $v \in \h$
    which implies that 
    $v(x) = 0$ for all $x \in \partial \Omega$.
    This proves part 2.

    We now use the above result to prove part 3. 
    To prove the second inequality
    we use 
    the fact that 
    the function $\nabla L$ 
    is Lipschitz,
    which implies that for all $x \in \Omega$
    we have 
    \begin{align*}
        \|\nabla L(\nabla u(x)) - \nabla L(\nabla v(x))\|_2 
            \leq \Lambda \|\nabla u(x) - \nabla v(x)\|_2
    \end{align*}
    Taking square on each side and itegrating over $\Omega$
    we get
    \begin{align*}
        \int_\Omega 
            \|\nabla L(\nabla u(x)) - \nabla L(\nabla v(x))\|_2^2dx 
        &\leq 
        \Lambda^2\int_\Omega \left\|\nabla u(x) - \nabla v(x)\right\|_2^2 dx \\
        \implies 
        \|\nabla L(\nabla u) - \nabla L(\nabla v)\|_{\ll}^2
            &\leq \Lambda^2\|\nabla u - \nabla v\|_{\ll}^2\\
        \implies 
        \|\nabla L(\nabla u) - \nabla L(\nabla v)\|_{\ll} 
            &\leq \Lambda\|\nabla u - \nabla v\|_{\ll}
    \end{align*}
    
    Hence, using Cauchy-Schwarz inequality we get,
    \begin{align*}
        \langle \nabla L(\nabla u) - \nabla L(\nabla v), \nabla u - \nabla v\rangle_{\ll}
        &\leq \|\nabla L(\nabla u) - \nabla L(\nabla v)\|_{\ll} \|\nabla u - \nabla v\|_{\ll} \\
        &\leq \Lambda \|\nabla u - \nabla v\|_{\ll} \|\nabla u - \nabla u\|_{\ll} \\
        &\leq \Lambda \|u - v\|_{\h}^2
    \end{align*}
    
    For the first inequality,
    we know that the function $F$ is strongly convex, i.e., 
    we have that 
    for all $x,y \in \R^d$
    we have
    \begin{align*}
        \left(\nabla L\left(\nabla u(x)\right) 
            - \nabla L\left(\nabla v(x)\right)\right)^T(\nabla u(x) - \nabla v(x)) 
        \geq \lambda \|\nabla u(x) - \nabla v(x)\|_{2}^2
    \end{align*}
    Integrating over $\Omega$ we get,
    \begin{align*}
        \int_\Omega \left(\nabla L\left(\nabla u(x)\right) 
            - \nabla L\left(\nabla v(x)\right)\right)^T
            (\nabla u(x) - \nabla v(x))  dx
        &\geq \lambda \int_\Omega \|\nabla u(x) - \nabla v(x)\|_{2}^2 dx \\
        \implies 
        \langle \nabla L(\nabla u) - \nabla L(\nabla v), \nabla u - \nabla v \rangle_{\ll}
        &\geq 
                \lambda \|\nabla u - \nabla v\|_{\ll}^2 \\
        \implies 
        \| \nabla L(\nabla u) - \nabla L(\nabla v)\|_{\ll}
        &\geq 
                \lambda \|\nabla u - \nabla v\|_{\ll} \\
    \end{align*}

    % For part $3.$ notice the following, 
    % \begin{align*}
    %     \sup_{w \in \h} \langle \op(w), w\rangle_{\ll}
    %     = \sup_{w \in \h} \langle -\divergence(\nabla L(\nabla w)), w\rangle_{\ll}
    % \end{align*}
    
    % \begin{align*}
    %     \|\op(w) - \op(v)\|_{\ll} 
    %     &= \sup_{\substack{\varphi \in \h \\ \|\varphi\|_{\h}=1}}
    %     \langle \op(w) - \op(v), \varphi \rangle_{\ll}\\
    %     &= 
    %     \sup_{\substack{\varphi \in \h \\ \|\varphi\|_{\h}=1}}
    %     \langle \nabla L(\nabla v) - \nabla L(\nabla w), \nabla \varphi \rangle_{\ll}\\
    %     &\leq 
    %     \sup_{\substack{\varphi \in \h \\ \|\varphi\|_{\h}=1}}
    %     \|\nabla L(\nabla w) - \nabla L(\nabla v)\|_{\ll}\|\nabla \varphi\|_{\ll}\\
    %     &\leq 
    %     \|\nabla L(\nabla w) - \nabla L(\nabla v)\|_{\ll} 
    %     \leq 
    %     \Lambda \|\nabla w - \nabla v\|_{\ll}
    % \end{align*}
    \qedhere
\end{proof}

\subsection{Proof for Lemma~\ref{lemma:I_minus_delta_inverse}}
\label{subsec:proof_of_I_minus_delta_invers}

\begin{proof}
    Let $\{\lambda_i,\varphi_i\}_{i=1}^\infty$
    denote the (eigenvalue, eigenfunction) pairs of the operator $\Delta$,
    where $\lambda_1 \leq \lambda_2 \leq \cdots$. 
    Furthermore, note that $\lambda_1 = \frac{1}{\pc}$.
    
    Now, let us write $v = \sum_i \mu_i \phi_i$.
    Notice that an eigenfunction of $\Delta$ is also an eigenfunction for $(I-\Delta)^{-1}$, 
    with correspondinding eigenvalue $\frac{1}{1+\lambda_i}$.
    
    To show part 1,
    we have,
    \begin{align*}
        \left\|\nabla (I -\Delta)^{-1} \nabla \cdot v\right\|_{\ll}^2
        &=
        \left\|(I - \Delta)^{-1} \Delta v\right\|_{\ll}^2 \\
        &= 
        \left\|\sum_{i=1}^\infty \frac{\lambda_i}{1 + \lambda_i}\mu_i \phi_i\right\|_{\ll}^2\\
        &\leq
        \left\|\sum_{i=1}^\infty \mu_i \phi_i\right\|_{\ll}^2\\
        &= \sum_{i=1}^\infty \mu_i^2 = \|u\|_{\ll}^2
    \end{align*}
    where we use the fact that $\phi_i$ are orthogonal.
    
    Now, 
    note that 
    $(I - \Delta)^{-1} v = \sum_{i=1}^\infty \frac{1}{(1 + \lambda_i)}\mu_i \phi_i$
    now, note that since $\lambda_1 \leq \lambda_2 \leq \cdots$
    we have for all $i\in \N$ 
    \begin{equation}
        \label{eq:l3_eq1}
        \frac{1}{1 + \lambda_i} \geq \frac{1}{C_p \lambda_i}
    \end{equation}
    and note that $\frac{1}{\lambda_i}$ are the eigenvalues for $\Delta^{-1}$ for all $i \in \N$.
    
    Now, bounding $\langle (I - \Delta)^{-1} v, v\rangle_{\ll}$
    \begin{align*}
        \langle (I - \Delta)^{-1} v, v\rangle_{\ll} 
            &= \left\langle \sum_{i=1}^\infty \frac{\mu_i}{1 + \lambda_i}\phi_i, 
                \sum_{i=1}^\infty \mu_i \phi_i \right\rangle_{\ll}\\
            &= \sum_{i=1}^\infty \frac{\lvert\mu_i\rvert^2}{1 + \lambda_i} \|\phi_i\|_{\ll}^2 \numberthis \label{eq:l3_eq2}
    \end{align*}
    where we the orthogonality of $\phi_i'$s to get \eqref{eq:l3_eq2}.
    Using the inequality in \eqref{eq:l3_eq1} we can further lower bound $\langle (I - \Delta)^{-1} v, v\rangle_{\ll}$
    as follows,
    \begin{align*}
        \langle (I - \Delta)^{-1} v, v\rangle_{\ll} 
            &\geq  \sum_{i=1}^\infty \frac{\lvert\mu_i\rvert^2}{\pc \lambda_i} \|\phi_i\|_{\ll}^2
            := \frac{1}{\pc}\langle \Delta^{-1} v, v\rangle_{\ll},
    \end{align*}
    where we use the following set of equalities in the last step,
    \begin{equation*} 
        \langle \Delta^{-1} v, v\rangle_{\ll} 
            = \left\langle \sum_{i=1}^\infty \frac{\mu_i}{\lambda_i} \phi_i, 
                \sum_{i=1}^\infty \mu_i\phi_i\right\rangle_{\ll} 
            = \sum_{i=1}^{\infty}\frac{\lvert\mu_i\rvert^2}{\lambda_i} \|\phi_i\|_{\ll}^2. \qedhere
    \end{equation*}
    % \begin{align*}
    %     (I - \Delta)^{-1} v 
    %     = \sum_{i=1}^\infty\frac{\mu_i}{1 + \lambda_i} \phi_i 
    %     \geq \sum_{i=1}^\infty \frac{\mu_i}{C_p \lambda_i} \phi_i 
    %     =: \Delta^{-1}v
    % \end{align*}
    % \jl{we can only conclude about the norm or the quadratic form here; the inequality above does not hold since $\phi_i$'s are not necessarily non-negative}
\end{proof}

\subsection{Proof for Convergence: 
Proof for Lemma~\ref{lemma:proof_for_convergence}}
\label{subsec:proof_of_proof_of_convergence}
\begin{proof}
    We show that the value of $\calE$ is decreasing as $t\to\infty$.
    
    For the analysis we consider 
    $\eta = \frac{\lambda^3}{\pc \Lambda^3}$
    For functions $u, \varphi \in \h$
    and $\varepsilon \in \R$, 
    since the function $L$ is smooth and convex,
    the following holds,
    % Note the following Taylor expansion of the energy functional,
    \begin{align*}
        \calE(\nabla u+ \varepsilon\nabla \varphi) 
        &= \int_\Omega L(\nabla u + \varepsilon \nabla \varphi) dx\\
        &\leq \int_\Omega\; L(\nabla u) + \varepsilon \nabla L(\nabla u) \nabla \varphi 
            + \frac{\varepsilon^2}{2} |\nabla \varphi|^2 \sup_{y \in \R^d} D^2L(y) dx\\
        &\leq \int_\Omega\; L(\nabla u) + \varepsilon \nabla L(\nabla u) \nabla \varphi 
            + \frac{\varepsilon^2\Lambda^2}{2} |\nabla \varphi|^2 dx\\
    \implies 
        \calE(\nabla u + \varepsilon\nabla \varphi) 
        &\leq \calE(\nabla u) + \varepsilon\langle \nabla L(\nabla u), \nabla \varphi\rangle_{\ll}
        + \frac{\varepsilon^2 \Lambda^2}{2}\|\nabla \varphi\|_{\ll}^2
        \numberthis \label{eq:taylor_expansion_of_energy_functional}
    \end{align*}
    We start with Taylor expanding the energy functional at step $t+1$
    around the function $u_{t+1}$, by using 
    \eqref{eq:taylor_expansion_of_energy_functional}
    and using $u = u_t$
    and $\varphi = - \op(u_t)$
    and $\varepsilon = \eta$ we get
    % Using $u=u_{t}$ and $$
    \begin{align*}
        \calE(u_{t+1}) 
        &\leq \calE(u_t) - \eta \underbrace{\left\langle \nabla L(\nabla u_t), 
            \nabla (I - \Delta)^{-1}\op(u_t)\right\rangle_{\ll}}_{\text{Term 1}}\\
        & \quad + \underbrace{\frac{\eta^2 \Lambda^2}{2} \left\|\nabla (I - \Delta)^{-1} \op(u_t)\right\|_{\ll}^2}_{\text{Term 2}}.
        \numberthis \label{eq:taylor_expansion_for_ut}
    \end{align*}
    
    First we lower bound \emph{Term 1.} 
    Note that since $u^\star$ is the solution to the PDE in \eqref{eq:non_linear_PDE_to_solve}
    we have $\op(u^\star)=0$.
    Furthermore, from the weak solution, i.e, 
    \eqref{eq:weak_solution} we have for all $\varphi \in \h$
    $\langle \nabla L(\nabla u^\star), \nabla \varphi\rangle_{\ll} = 0$, 
    hence, we also have 
    $\langle \nabla L(\nabla u^\star), \nabla (I - \Delta)^{-1} \op(u_t)\rangle_{\ll} = 0$, 
    which is a bilinear form that we can subtract from Term 1.
    Therefore we have
    \begin{align*}
        &\left\langle \nabla L (\nabla u_t), \nabla (I - \Delta)^{-1} \op(u_t)\right\rangle_{\ll}\\
        &= \left\langle \nabla L (\nabla u_t) - \nabla L(\nabla u^\star), \nabla (I - \Delta)^{-1} \left(\op(u_t) - \op(u^\star)\right)\right\rangle_{\ll}\\
        &= \int_\Omega \left(\nabla L(\nabla u_t)  - \nabla L(\nabla u^\star) \right) 
            \cdot \nabla (I - \Delta)^{-1} \nabla \cdot \left(\nabla L(\nabla u_t) 
            - \nabla L(u^\star)\right)dx\\
        &\stackrel{(i)}{\geq} \frac{1}{\pc}\int_\Omega \left(\nabla L(\nabla u_t) - \nabla L(\nabla u^\star) \right)
            \cdot \nabla \Delta^{-1} \nabla \cdot \left(\nabla L(\nabla u_t) - \nabla L(\nabla u^\star)\right) dx\\
        % &= \int_\Omega \nabla L(\nabla u_t)  \cdot \nabla L(\nabla u_t) dx\\
        &\geq \frac{1}{\pc}\langle \nabla L(\nabla u_t)  - \nabla L(\nabla u^\star), \nabla L(\nabla u_t) - \nabla L(\nabla u^\star) \rangle_{\ll} \\
        &\geq \frac{\lambda^2}{\pc} \|\nabla u_t - \nabla u^\star\|_{\ll}^2 
        \\ & \geq \frac{\lambda^2}{\pc \Lambda} \left(\calE(u_t) - \calE(u^\star)\right)
        \numberthis \label{eq:lower_bound_for_term1}
    \end{align*}
    where we use 
    the result from 
    Lemma~\ref{lemma:I_minus_delta_inverse} (part $2.$)
    in $(i)$,
    and the results from Lemma~\ref{lemma:properties_of_EandL} (parts \emph{4.} and \emph{1.}, respectively).
    
    Furthermore, we can bound \emph{Term 2} using result from Lemma~\ref{lemma:I_minus_delta_inverse}
    (part \emph{1.}) such that,
    \begin{align*}
        \left\|\nabla (I - \Delta)^{-1} \op(u_t)\right\|_{\ll}^2 
        &= \left\|\nabla (I - \Delta)^{-1} \left(\op(u_t) - \op(u^\star)\right)\right\|_{\ll}^2  \\
        &= \left\|\nabla (I - \Delta)^{-1} \nabla \cdot 
            \left(\nabla L(\nabla u_t) - \nabla L(\nabla u^\star)\right)\right\|_{\ll}^2 \\
        &\leq \left\|\nabla L(\nabla u_t) - \nabla L(\nabla u^\star)\right\|_{\ll}^2 \\
        &\leq \Lambda^2 \left\|\nabla u_t - \nabla u^\star\right\|_{\ll}^2 \\
        &\leq \frac{\Lambda^2}{\lambda} \left(\calE(u_t) - \calE(u^\star)\right).
        \numberthis \label{eq:lower_bound_for_term2}
    \end{align*}
    
    Using the results from \eqref{eq:lower_bound_for_term1}
    and \eqref{eq:lower_bound_for_term2}
    in \eqref{eq:taylor_expansion_for_ut}
    to get,
    \begin{align*}
        \implies \calE(u_{t+1}) - \calE(u^\star)  \leq \calE(u_t) - \calE(u^\star) - \left(\frac{\lambda^2}{\pc \Lambda} 
                            - \eta \frac{\Lambda^2}{2\lambda}\right)\eta \left(\calE(u_t) - \calE(u^\star)\right)
    \end{align*}
    % where we use the fact that $\calE(u^\star) = 0$ from Assumption~\ref{assumption:1}.
    
    Since $\eta = \lambda^3/(\pc \Lambda^3)$
    we have
    \begin{align*}
        % &\calE(u_{t+1}) -\calE(u^\star) \leq \calE(u_t) - \frac{\lambda^2}{2\pc \Lambda}\eta\left(\calE(u_t) - \calE(u^\star)\right)\\
        % \implies&
        % \calE(u_{t+1})-\calE(u^\star) 
        %     \leq \left(1 - \frac{\lambda^2\eta}{2\pc \Lambda}\right)^t\left(\calE(u_0) - \calE(u^\star)\right)
        &\calE(u_{t+1}) -\calE(u^\star) \leq \calE(u_t) - \frac{\lambda^5}{2\pc \Lambda^4}\eta\left(\calE(u_t) - \calE(u^\star)\right)\\
        \implies&
        \calE(u_{t+1})-\calE(u^\star) 
            \leq \left(1 - \frac{\lambda^5}{2\pc \Lambda^4}\right)^t\left(\calE(u_0) - \calE(u^\star)\right). \qedhere
    \end{align*}
\end{proof}
