# Supplementary material for: Neural Network Approximations of PDEs Beyond Linearity: A Representational Perspective
Source: arXiv:2210.12101 source file (2023-03-27)
Supplement: Supplementary file 5 [file poincare.tex]

\subsection{
Proof of Corollary~\ref{corollary:equivalence}:
Equivalence of $\h$ and $\hh$ norms
}
\label{subsec:proof_for_poincare_corollary}

\begin{proof}
    Note that for $u \in \h$ we have, 
    \begin{align*}
        \|u\|_{\hh} &= \|\nabla u\|_{\ll} + \|u\|_{\ll} \\
        &\geq \|\nabla u\|_{\ll} \\
        \implies \|u\|_{\hh} &\geq \|u\|_{\h}.  
        % \numberthis \label{eq:H_01_lbd_H_1}
    \end{align*}
    Where we have used the definition of the norm in $\h$ space. 
    
    Further, using the result in Theorem \ref{thm:poincare_inequality} 
    we have
    \begin{align*}
        \|u\|^2_{\hh} = 
            \left(\|u\|^2_{\ll} + \|\nabla u\|^2_{L^2(\Omega)}\right) 
            \leq \left(C_p^2 + 1\right)\|\nabla u\|^2_{\hh}
        \numberthis \label{eq:upd_H1_H_0_1}
    \end{align*}
    Therefore, 
    % combining the results from (\ref{eq:upd_H1_H_0_1}) and (\ref{eq:H_01_lbd_H_1}) we have
    combining the two inequalities we have
    \begin{equation}
        \label{eq:relation_H_01_H_1}
        \|u\|_{\h} \leq \|u\|_{\hh} \leq C_h\|u\|_{\h}
    \end{equation}
    where $C_h = (C_p^2  + 1)$.
    Hence we have that the norm in $\h$ and $\hh$ spaces are equivalent.
\end{proof}
